# Supplementary material for: SEAGLE - I: A pipeline for simulating and modeling strong lenses from cosmological hydrodynamic simulations
Source: arXiv:1802.06629 source file (2018-06-29)
Supplement: Supplementary file 1 [file appendix.tex]

\appendix \label{app}

\section{Some relevant Details}\label{eagleapp}

\begin{figure*}
	
\includegraphics[width=\textwidth]{pipeline}
\caption{The entity-relationship diagram for the SEAGLE database. Entities (tables) are connected to each other by relations, such as corresponds to or has. Relations can have degrees, e.g. one-to-one (1,1), one-to-many (1,N), or none-to-many (0,N). We have used the Crow’s foot and the (min,max)-notation to denote relationships on the diagram. The tick mark shows the starting point of the pipeline.} \label{pipe}
\end{figure*}

\begin{figure*}
\includegraphics[width=\textwidth]{H1S0Bobs_final_image_tri_L}
\caption{Lens parameters obtained from {\tt LENSED}: The model parameters of a lens obtained for a lens simulated from a typical early type galaxy ($\rm M_{*} = 9.14\times10^{11}M_{\odot}$ shows efficient convergence. The parameter space includes SIE lens profile with lens position ($x_L$, $y_L$), Einstein radius ($r_L$), axis ratio ($q_L$), position angle ($\phi_L$) and shear vector components ($\gamma_1$ and $\gamma_2$). This lens-modeling is done with 200 live points. }\label{lens}
\end{figure*}

\begin{figure*}
\includegraphics[width=\textwidth]{H1S0Bobs_final_image_tri_S}
\caption{Source parameters obtained from {\tt LENSED}: The model parameters of a lens created from a typical early type galaxy ($\rm M_{*} = 9.14\times10^{11}M_{\odot}$) shows efficient convergence. The parameter space includes S\'{e}rsic source profile with source position ($x_S$, $y_S$), source size ($r_S$), axis ratio ($q_S$), position angle ($\phi_S$), source index ($n_S$) and scaled source magnitude ($mag_S$). The actual source magnitude could be obtained by subtracting $mag_S$ from the background magnitude in the filed of view of the image. Here we show an example of the corner plot of the source modeling.}\label{source}
\end{figure*}
